# Supplementary material for: MINN: Learning the dynamics of differential-algebraic equations and application to battery modeling
Source: arXiv:2304.14422 source file (2025-01-30)
Supplement: Supplementary file 1 [file supplement.pdf]

# MINN: Learning the Dynamics of Differential-Algebraic Equations and Application to Battery Modeling

## Supplementary Material

Yicun Huang<sup>a</sup>, Changfu Zou<sup>a,\*</sup>, Yang Li<sup>a</sup>, Torsten Wik<sup>a,\*</sup>

<sup>a</sup>Department of Electrical Engineering, Chalmers University of Technology, Gothenburg, 412 96, Sweden

Table 1: Electrochemical parameters of the lithium-ion battery model used in generating synthetic data for training.

| Parameter             | Pos                    | Sep                 | Neg                   | Meaning                                                                             |
|-----------------------|------------------------|---------------------|-----------------------|-------------------------------------------------------------------------------------|
| $\delta$              | $75.6 \times 10^{-6}$  | $12 \times 10^{-6}$ | $85.2 \times 10^{-6}$ | Thickness [m]                                                                       |
| $R$                   | $5.22 \times 10^{-6}$  | –                   | $5.86 \times 10^{-6}$ | Particles' radius [m]                                                               |
| $C_s^{\max}$          | 51,765                 | –                   | 29,583                | Max solid concentration [ $\text{mol}\cdot\text{m}^{-3}$ ]                          |
| $C_s^{0\%}$           | 47,023                 | –                   | 825                   | Min concentration at SOC 0%                                                         |
| $C_s^{100\%}$         | 13,774                 | –                   | 26,666                | Max concentration at SOC 100%                                                       |
| $k_0$                 | $3.54 \times 10^{-11}$ | –                   | $3.3 \times 10^{-14}$ | Reaction rate constant [ $\text{m}^{2.5}\cdot\text{mol}^{-0.5}\cdot\text{s}^{-1}$ ] |
| $D_s$                 | $4.0 \times 10^{-15}$  | –                   | $1.6 \times 10^{-14}$ | Solid diffusion [ $\text{m}^2\cdot\text{s}^{-1}$ ]                                  |
| $\sigma_{\text{eff}}$ | $9.76 \times 10^{-2}$  | –                   | 139.65                | Solid conductivity [ $\text{S}\cdot\text{m}^{-1}$ ]                                 |
| $a_s$                 | 382,183                | –                   | 383,959               | Specific interfacial surface area [ $\text{m}^{-1}$ ]                               |
| $R_{\text{SEI}}$      | 0.01                   | –                   | 0.025                 | SEI resistance [ $\Omega\cdot\text{m}^{-1}$ ]                                       |
| $\epsilon_e$          | 0.335                  | 0.47                | 0.25                  | Porosity                                                                            |

### Electrochemical Parameterization

Most parameterizations of the pseudo-two-dimensional (P2D) model [1] in the literature follow global optimization techniques and are based on full-cell measurements, which are unlikely to yield a globally optimal solution of all the parameters [2, 3]. For the generation of faithful synthetic data, multi-step parameterization based on half-cell measurements has previously been conducted for an LG M50 cell with Nickel-Manganese-Cobalt (NMC) 111 chemistry [4]. This work adopts the available parameters with a minor change to the aging-related parameters,  $R_{\text{SEI}}$ , in order to simulate the behavior of aged cells. The values of the corresponding electrochemical parameters and constants are listed in Tables 1 and 2, respectively.

\*Corresponding authors. Address: Hörsalsvägen 11, SE-412 96 Gothenburg, Sweden.

Table 2: Electrochemical constants of the lithium-ion battery model used in generating synthetic data for training.

| Constant         | Value                  | Meaning                                                                   |
|------------------|------------------------|---------------------------------------------------------------------------|
| $C_e^0$          | 1000                   | Electrolyte initial concentration [mol·m <sup>-3</sup> ]                  |
| $t_+$            | 0.2594                 | Transference number                                                       |
| Burrg            | 1.5                    | Bruggeman constant                                                        |
| $\alpha$         | 0.5                    | Symmetry factor                                                           |
| $T_{\text{ref}}$ | 298.15                 | Reference temperature [K]                                                 |
| $F$              | 96487                  | Faraday constant [C·mol <sup>-1</sup> ]                                   |
| $k_B$            | $1.38 \times 10^{-23}$ | Boltzmann constant [m <sup>2</sup> ·kg·s <sup>-2</sup> ·K <sup>-1</sup> ] |
| $Q_n$            | 5                      | Nominal capacity [Ah]                                                     |
| $A_s$            | 0.1027                 | Electrode active surface area [m <sup>2</sup> ]                           |

The expressions of effective electrolyte diffusion coefficient  $D_e^{\text{eff}}$  and effective electrolyte conductivity  $\kappa_{\text{eff}}$  as functions of electrolyte concentration are obtained from [4]:

$$D_e^{\text{eff}} = 8.794 \times 10^{-11} \left( \frac{C_e}{C_e^0} \right)^2 - 3.972 \times 10^{-10} \frac{C_e}{C_e^0} + 4.862 \times 10^{-10},$$

$$\kappa_{\text{eff}} = 0.1297 \left( \frac{C_e}{C_e^0} \right)^3 - 2.51 \left( \frac{C_e}{C_e^0} \right)^{1.5} + 3.329 \left( \frac{C_e}{C_e^0} \right).$$

With  $\xi := C_s^R / C_s^{\text{max}}$ , the open circuit potential (OCP) of an NMC111 electrode is given by

$$\begin{aligned} \text{OCP}_{\text{cathode}} = & -0.8090\xi + 4.4875 - 0.0428 \tanh(18.5138(\xi - 0.5542)) \\ & - 17.7326 \tanh(15.7890(\xi - 0.3117)) + 17.5842 \tanh(15.9308(\xi - 0.3120)), \end{aligned}$$

and the OCP of a graphite electrode:

$$\begin{aligned} \text{OCP}_{\text{anode}} = & 5.38 \exp(-39.3631\xi) + 0.2482 - 0.0909 \tanh(29.8538(\xi - 0.1234)) \\ & - 0.04478 \tanh(14.9159(\xi - 0.2769)) - 0.0205 \tanh(30.4444(\xi - 0.6103)). \end{aligned}$$

The grouping of parameters in the MINN battery model facilitates the development of aging-adaptive battery models. In Table 3, aging-related parameters are listed along with their locations in the MINN formulation. These parameters are unexpected to change during battery lifetime due to various parasitic side reactions, whereas other parameters involved in the approximation of  $G_{\text{NN}}$  are invariant compared with aging-related parameters.

Table 3: Ageing-related parameters in the MINN formulation. These parameters are not fixed during learning.

| Ageing-related parameters | Location               |
|---------------------------|------------------------|
| $R_{\text{SEI}}$          | Output function $Y(h)$ |
| $\epsilon_e$              | $f(h_d, I)$            |
| $D_e^{\text{eff}}$        | $f(h_d, I)$            |
| $D_s$                     | $f(h_d, I)$            |
| $k_0$                     | $f(h_d, I)$            |

## Numerical Methods

The spatial discretization employed in this work, encompassing both data generation and the construction of the physics-based equations in the MINN framework, utilizes a spectral collocation method. This method is known for its spectral accuracy when the solution to be approximated is sufficiently smooth. Consequently, it enables the reduction in the number of states required in the differential-algebraic equations (DAEs) for evaluating the infinite-dimensional partial differential-algebraic equations (PDAEs). We consider this choice of discretization to be a numerical technique rather than an intrinsic characteristic of the MINN framework.

The spectral method starts with a finite sum approximation of the solution by using orthogonal basis functions:

$$u_N(x, t) = \sum_{k=0}^N \hat{u}_k(t) \mathcal{P}(x) \quad x \in [-1, 1], \quad (1)$$

which approximates a field of spatial-temporal coordinate  $(x, t)$  by  $N + 1$  grid points, e.g.  $C_e(x, t)$ . The polynomials  $\mathcal{P}(x)$  used in this work are Chebyshev polynomials for the non-periodic boundary conditions seen in the electrochemical formulation of the battery.

In the implementation, the physical domain is transformed to  $[-1, 1]$ . The coefficients  $\hat{u}_k(t)$  are determined by substituting (1) into the partial differential equations. Take the electrolyte diffusion equation in the anode, for example,

$$\epsilon_e \frac{\partial C_e}{\partial t} = \frac{\partial}{\partial x} \left( D_e^{\text{eff}}(C_e) \frac{\partial C_e}{\partial x} \right) + a_s (1 - t_+^0) j, \quad (2)$$

$$\frac{\partial C_e}{\partial t} = \frac{D_e^{\text{eff}}}{\epsilon_e} \frac{\partial^2 C_e}{\partial x^2} + \frac{1}{\epsilon_e} \frac{\partial D_e^{\text{eff}}}{\partial C_e} \left( \frac{\partial C_e}{\partial x} \right)^2 + \frac{a_s (1 - t_+^0) j}{\epsilon_e}. \quad (3)$$

Here,  $\partial D_e^{\text{eff}} / \partial C_e$  is a function of  $C_e$  for which we denote by  $f_{dc}$ , and  $a_s(1 - t_+^0)j/\epsilon_e$  term can be treated as a constant at a given time  $t$ . By exploring the properties of (1) at some specially chosen grid points, the spatial derivatives of  $C_e$  can be

written in matrix forms [5], i.e.  $\partial^2 C_e / \partial x^2 = \mathcal{D}^2 C_e$  and  $\partial C_e / \partial x = \mathcal{D} C_e$ , where  $\mathcal{D}$  is the first Chebyshev differentiation matrix on  $[-1, 1]$ . By this approximation, Eqn. (3) becomes a vector-valued ordinary differential equation for the electrolyte concentration values  $C_{e,k}(t)$  at grid point  $k$ ,

$$\frac{dC_{e,k}(t)}{dt} = \frac{D_e^{\text{eff}}}{\epsilon_e} \mathcal{D}^2 C_{e,k}(t) + \frac{1}{\epsilon_e} f_{dc}(C_{e,k}(t)) (\mathcal{D} C_{e,k}(t))^2 + \frac{a_s (1 - t_+^0) j(t)}{\epsilon_e}. \quad (4)$$

Eqns. (4) are solved for  $N - 1$  inner grid points, and the boundary nodes are, in turn, calculated from the inner grid points using boundary conditions.

For the time integration, the solver used in this work employs a multistage implicit scheme suited for stiff systems. The scheme for computing the hidden state  $h_d$  at time step  $k + 1$  is given by:

$$h_d^{k+1} = h_d^k + \delta t^k \sum_{i=1}^s b_i d_i, \quad (5)$$

where  $h_d^k$  and  $\delta t^k$  are the solution and step size at time step  $k$ , respectively,  $s$  is the number of stages,  $d_i$  are the stage derivatives, and  $b_i$  are the weights associated with each stage  $i$ . Because of stiffness issues, an implicit scheme requires that the evaluation of stage derivatives involves the solution at the next time step. For this reason, a stiff ODE solver solves (5) iteratively at each time step.

### Model Evaluation under 1C Charge

The internal states are important for battery modeling. Inaccurate prediction of their values will inevitably lead to under- or over-utilization of the battery capacity and energy. For example, in model predictive control, the constraint may be set to a lower bound of the plating potential at the anode-separator interface in a fast-charging scenario. Fig. 1d–f shows the plating potential predictions of different models, including our proposed MINN model and its counterparts, i.e., P2D and neural ODE (NODE). These models are trained at 30% SOC and tested at 50% SOC here for comparison. It can be seen in Fig. 1h that the MINN model outperformed NODE in its predictive accuracy. Likewise, the electrolyte concentration plots in Fig. 1a–c present another important internal state, which can be depleted during charging. Fig. 1h shows the root mean square error (RMSE) of the electrolyte concentration measured in mV. The DNN and PINN models appearing in Fig. 5 of the main document are not suitable for comparison here because they cannot handle different initializations from those used in training.

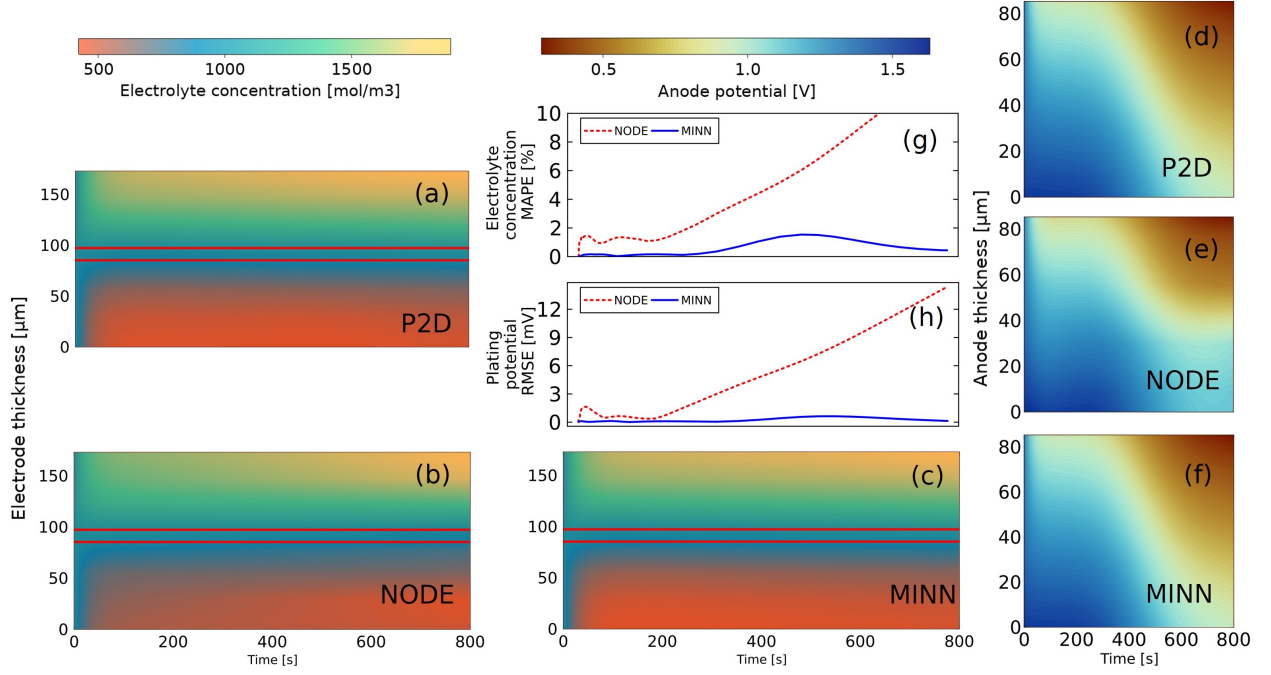

Figure 1: (a)–(c) Spatiotemporal plots of the electrolyte concentration predicted by different battery models starting from 50% SOC, where the top of each sub-figure represents the cathode and the bottom signifies the anode. (d)–(f) Spatiotemporal plots of the plating potential for the models. (g)–(h) The errors of the NODE and MINN models in reference to the P2D ground truth.

### Model Evaluation under A Driving Cycle

In the main document, Fig. 7 shows the results of the testing data at a SOC range of 85–90%. It has been shown that other SOC ranges yield similar results in predicting the model outputs and internal states. For example, Fig. 2 shows the benchmarks of the internal states, including the electrolyte concentration and surface concentration. Both models involved in the benchmark, including the DD-ROM and MINN, yield accurate predictions compared with the P2D ground truth. Similarly, Fig. 3 shows the predictions of the outputs, i.e., the terminal voltage and the plating potential at the anode-separator interface. Both models perform very well for the driving cycle.

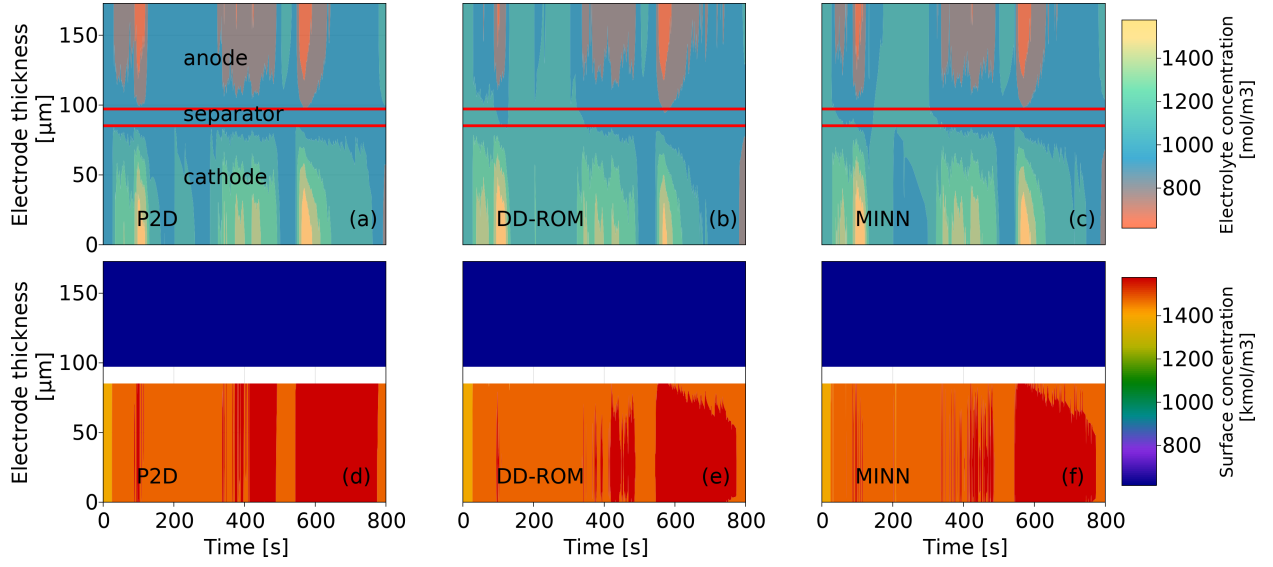

Figure 2: Performance of the DD-ROM and MINN battery models in learning battery internal states, compared with that of the reference, i.e., the 144-order P2D model. (a)-(c) Liquid-phase ion concentration (electrolyte concentration). (d)-(f) Solid-phase concentration at the surface of particles.

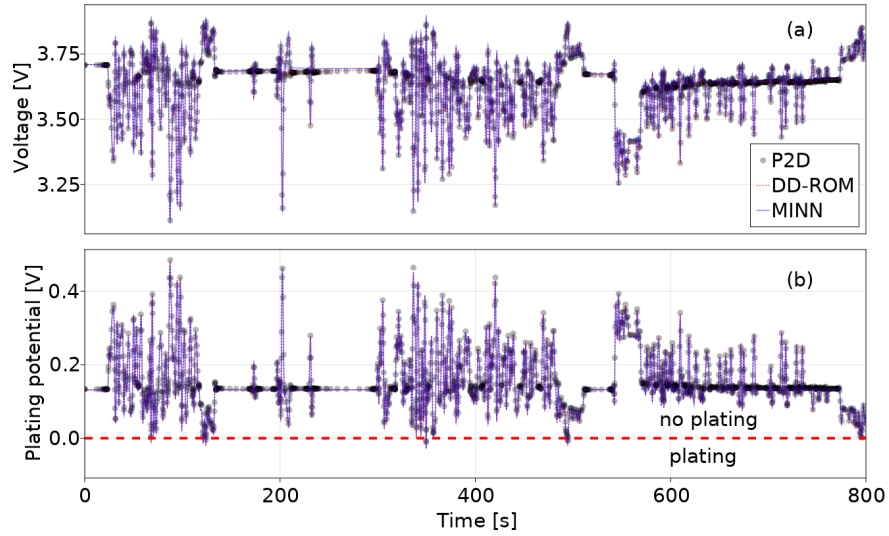

Figure 3: Results of the DD-ROM and MINN battery models in learning battery outputs, compared with those of the 144-order P2D model. (a) Terminal voltage response to the testing current. (b) Anode plating potential at the anode-separator interface.

## References

- [1] T. F. Fuller, M. L. Doyle, J. Newman, Simulation and optimization of the dual lithium ion insertion cell, *J. Electrochem. Soc.* 141 (1994) 1–10.
- [2] Z. Khalik, M. Donkers, J. Sturm, H. Bergveld, Parameter estimation of the Doyle-Fuller-Newman model for lithium-ion batteries by parameter normalization, grouping, and sensitivity analysis, *J. Power Sources* 499 (2021) 229901.

- [3] W. Li, D. Cao, D. Jöst, F. Ringbeck, M. Kuipers, F. Frie, D. U. Sauer, Parameter sensitivity analysis of electrochemical model-based battery management systems for lithium-ion batteries, *Appl. Energy* 269 (2020) 115104.
- [4] C.-H. Chen, F. B. Planella, K. B. O'Regan, D. Gastol, W. D. Widanage, E. Kendrick, Development of experimental techniques for parameterization of multi-scale lithium-ion battery models, *J. Electrochem. Soc.* (2020).
- [5] L. N. Trefethen, *Spectral Methods in MATLAB*, Society for Industrial and Applied Mathematics, 2000.
